# Supplementary material for: Bootstrapping a User-Centered Task-Oriented Dialogue System
Source: arXiv:2207.05223 source file (2022-07-21)
Supplement: Supplementary file 1 [file Appendix.tex]

%auto-ignore
\section*{Appendix}
\section{Intent Scheme}
\label{apdx:intent_scheme}
\noindent\textbf{Sentiment.} At each turn, the user may confirm or reject the response of the bot. Accordingly, we have three intents \texttt{Affirm}, \texttt{Negate} and \texttt{Neutral} to identify the polarity of the user utterance.

\noindent\textbf{Navigation.} In the Task Catalog state, users can use \texttt{More/Less Choice} intents to view candidate tasks. In Task Execution, we support navigation commands including \texttt{Forward (X Steps)}, \texttt{Backward (X Steps)}, and \texttt{Go To Step X}, where \texttt{X} is a number specified by the user.

\noindent\textbf{Question.} The user may ask various questions throughout the conversation. Once the \texttt{Question} intent is detected, the user utterance will be passed to the question answering module.

\noindent\textbf{Task Request.} When users are looking for a task.
%Recognize task request initiated by the user and call the searching module.

\noindent\textbf{Detail Request.} Request details of a step.

\noindent\textbf{Repeat.} Repeat the previous response.

\noindent\textbf{Help.} Request help information that explains how to interact with the bot in each dialogue state.

\noindent\textbf{Stop.} Terminate the ongoing conversation.

\noindent\textbf{Timer.} We support Alexa timer management features, such as \texttt{Set}, \texttt{Pause}, \texttt{Resume}, and \texttt{Cancel} the timer.

\noindent\textbf{List.} We support Alexa list management features, such as \texttt{Add} and \texttt{Remove} items.

\noindent\textbf{Ignore.} Any user input that does not change dialogue states, such as incomplete utterance, greetings from the user, etc.

%\section{WikiHow Question-Answer Pair Annotation Protocol}
\section{In-context QA Annotation Example}
\label{apdx:qa_anno_protocol}

…\\
\textit{\textbf{Context:}} Step 3: Blanch the tomatoes. Drop a few tomatoes into the boiling water. Let them blanch for about 30 seconds. Remove the tomatoes and place them on a cutting board to cool. Repeat with the remaining tomatoes. Don't leave the tomatoes in the water too long. Blanching loosens their skins, but leaving them in the pot for more than 30 seconds will cause them to actually start cooking, which will make them lose their flavor. Be careful when removing the tomatoes from the boiling water. The best tools to use are tongs or a large slotted spoon.\\

\textit{\textbf{Question1:}}  Sorry, how long for blanching? \\
\textit{\textbf{Answer1:}}  Let them blanch for about 30 seconds.\\

\textit{\textbf{Question2:}}  Alexa, what tools should I use to remove the tomatoes from the boiling water?\\
\textit{\textbf{Answer2:}}  The best tools to use are tongs or a large slotted spoon.\\

\textit{\textbf{Question3:}}  What if I leave the tomatoes in the water too long?\\
\textit{\textbf{Answer3:}}  [No Answer]\\
…
